# Supplementary material for: A Unified Study of LoRA Variants: Taxonomy, Review, Codebase, and Empirical Evaluation
Source: arXiv:2601.22708 source file (2026-01-30)
Supplement: Supplementary file 1 [file appendix.tex]

\documentclass[9.5pt,journal]{IEEEtran}
\setlength{\baselineskip}{11.5pt}
\usepackage{booktabs}    
\usepackage{amsmath,amsfonts}
\allowdisplaybreaks 
\usepackage{algorithmic}
\usepackage{array}
\usepackage{hyperref}
\usepackage{tabularx} % For adjustable column width
\usepackage[caption=false,font=normalsize,labelfont=sf,textfont=sf]{subfig}
\usepackage{textcomp}
\usepackage{stfloats}
\usepackage{url}
\usepackage{verbatim}
\usepackage{graphicx}
\usepackage{mathtools}
\usepackage{pifont}
\usepackage{tikz}
\usepackage{cite}
\usepackage{graphicx}
\usepackage{forest}
\usepackage{listings}
\usepackage{xcolor}
\usepackage{graphicx}
\usepackage{amssymb}

\usepackage[table]{xcolor} 
% 设置代码样式
\lstset{
    language=Python,
    basicstyle=\ttfamily\small,
    keywordstyle=\color{blue},
    commentstyle=\color{gray}\itshape,
    stringstyle=\color{red},
    showstringspaces=false,
    breaklines=true,
    frame=single,
    numbers=left,
    numberstyle=\tiny\color{gray},
    tabsize=4
}
\forestset{
  forked edges/.style={
    for tree={
      grow=east,
      parent anchor=east,
      child anchor=west,
      edge path'={
        (!u.parent anchor) -- +(5pt,0) |- (.child anchor)
      },
      if level=0{}{
        if={n==1}{edge path'={(!u.parent anchor) -- +(5pt,0) |- (.child anchor)}}{}
      }
    }
  }
}

  % 绿色勾
   % 红色叉

\hyphenation{op-tical net-works semi-conduc-tor IEEE-Xplore}
\def\BibTeX{{\rm B\kern-.05em{\sc i\kern-.025em b}\kern-.08em
    T\kern-.1667em\lower.7ex\hbox{E}\kern-.125emX}}
\usepackage{balance}
\begin{document}
\author{
}
% \author{}

\markboth{Journal of \LaTeX\ Class Files,~Vol.~18, No.~9, September~2020}%
{How to Use the IEEEtran \LaTeX \ Templates}

\input{Sections/E.Appendix}
\clearpage
\bibliographystyle{IEEEtran}
\bibliography{reference}
\clearpage
\end{document}
